# Supplementary material for: Safe and Reliable Training of Learning-Based Aerospace Controllers
Source: arXiv:2407.07088 source file (2024-07-09)
Supplement: Supplementary file 1 [file 99appendix.tex]

%\appendix
\setcounter{section}{0}

\clearpage
{\huge{Appendix}}

\section{DNN Architecture \& Training}
\label{sec:appendix:DnnTraining}

%2D Spacecraft Docking Safe Reinforcement Learning Benchmark task \cite{ravaioli2022safe}. In this scenario, the agent (deputy MRDGE) spacecraft controlled with fixed thrusters attempts to safely maneuver into close proximity with a chief spacecraft while obeying a distance dependent safety constraint.
%\subsubsection{Dynamics Model}
%The system is modeled using Clohessy-Wiltshire relative orbital motion linear approximation in the non-inertial Hill's reference frame with the chief spacecraft lying at the origin \cite{clohessy1960terminal, hill1878researches}. The state of the system, $\boldsymbol{x} = [x, y, \dot{x}, \dot{y}]^T$, is defined as the x, y position and velocities

% Ieva
\begin{figure}[h]
    \centering
    %plots/docking_general_plot.pdf
    \includegraphics[width=0.9\textwidth]{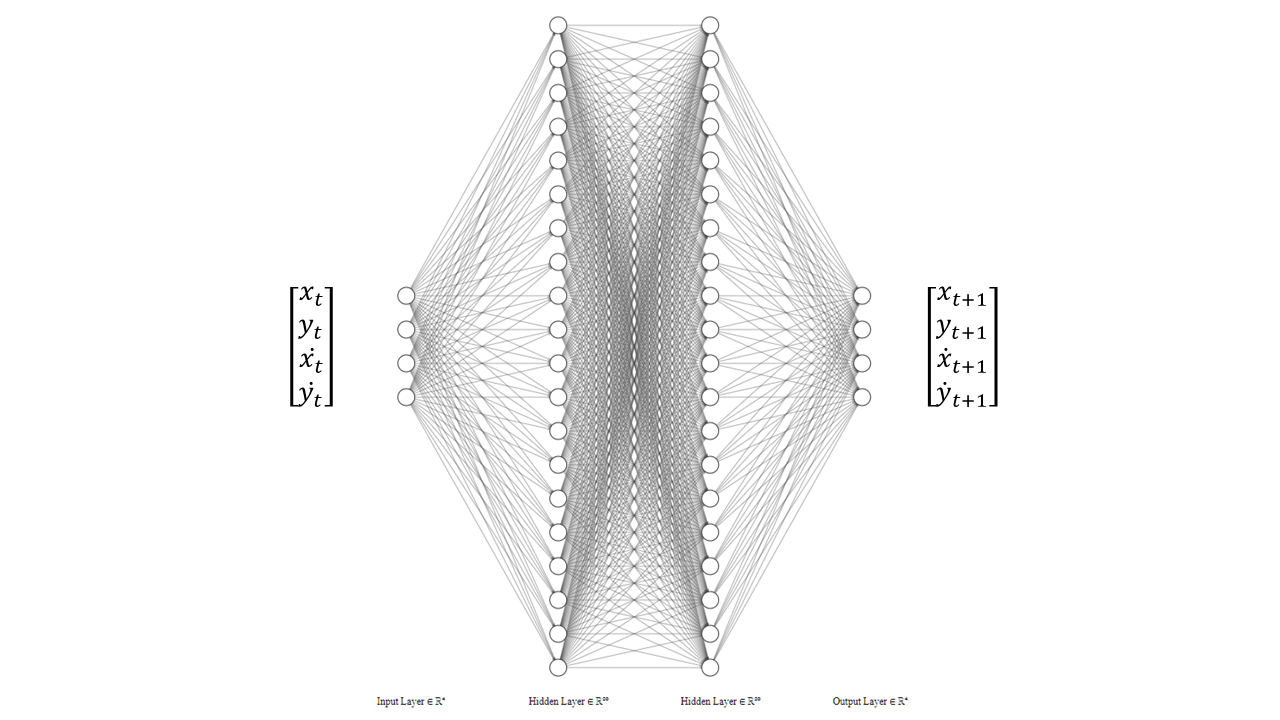}
    \caption{Controller neural network architecture for the 2D Spacecraft Docking Safe Reinforcement Learning Benchmark task. Given an input state of the system, $\boldsymbol{x} = [x_{t}, y_{t}, \dot{x_{t}}, \dot{y_{t}}]^T$, predict the next state per time step, such that the the agent spacecraft attempts to safely maneuver into close proximity with a chief spacecraft.}
    \label{fig:docking_general_plot_new}
\end{figure}

\newpage
\section{Failed Verification Attempts}
\label{sec:appendix:failedVerificationAttepts}

Our failed attempts include...

\begin{figure}[h]
    \centering
    \includegraphics[width=0.6\textwidth]{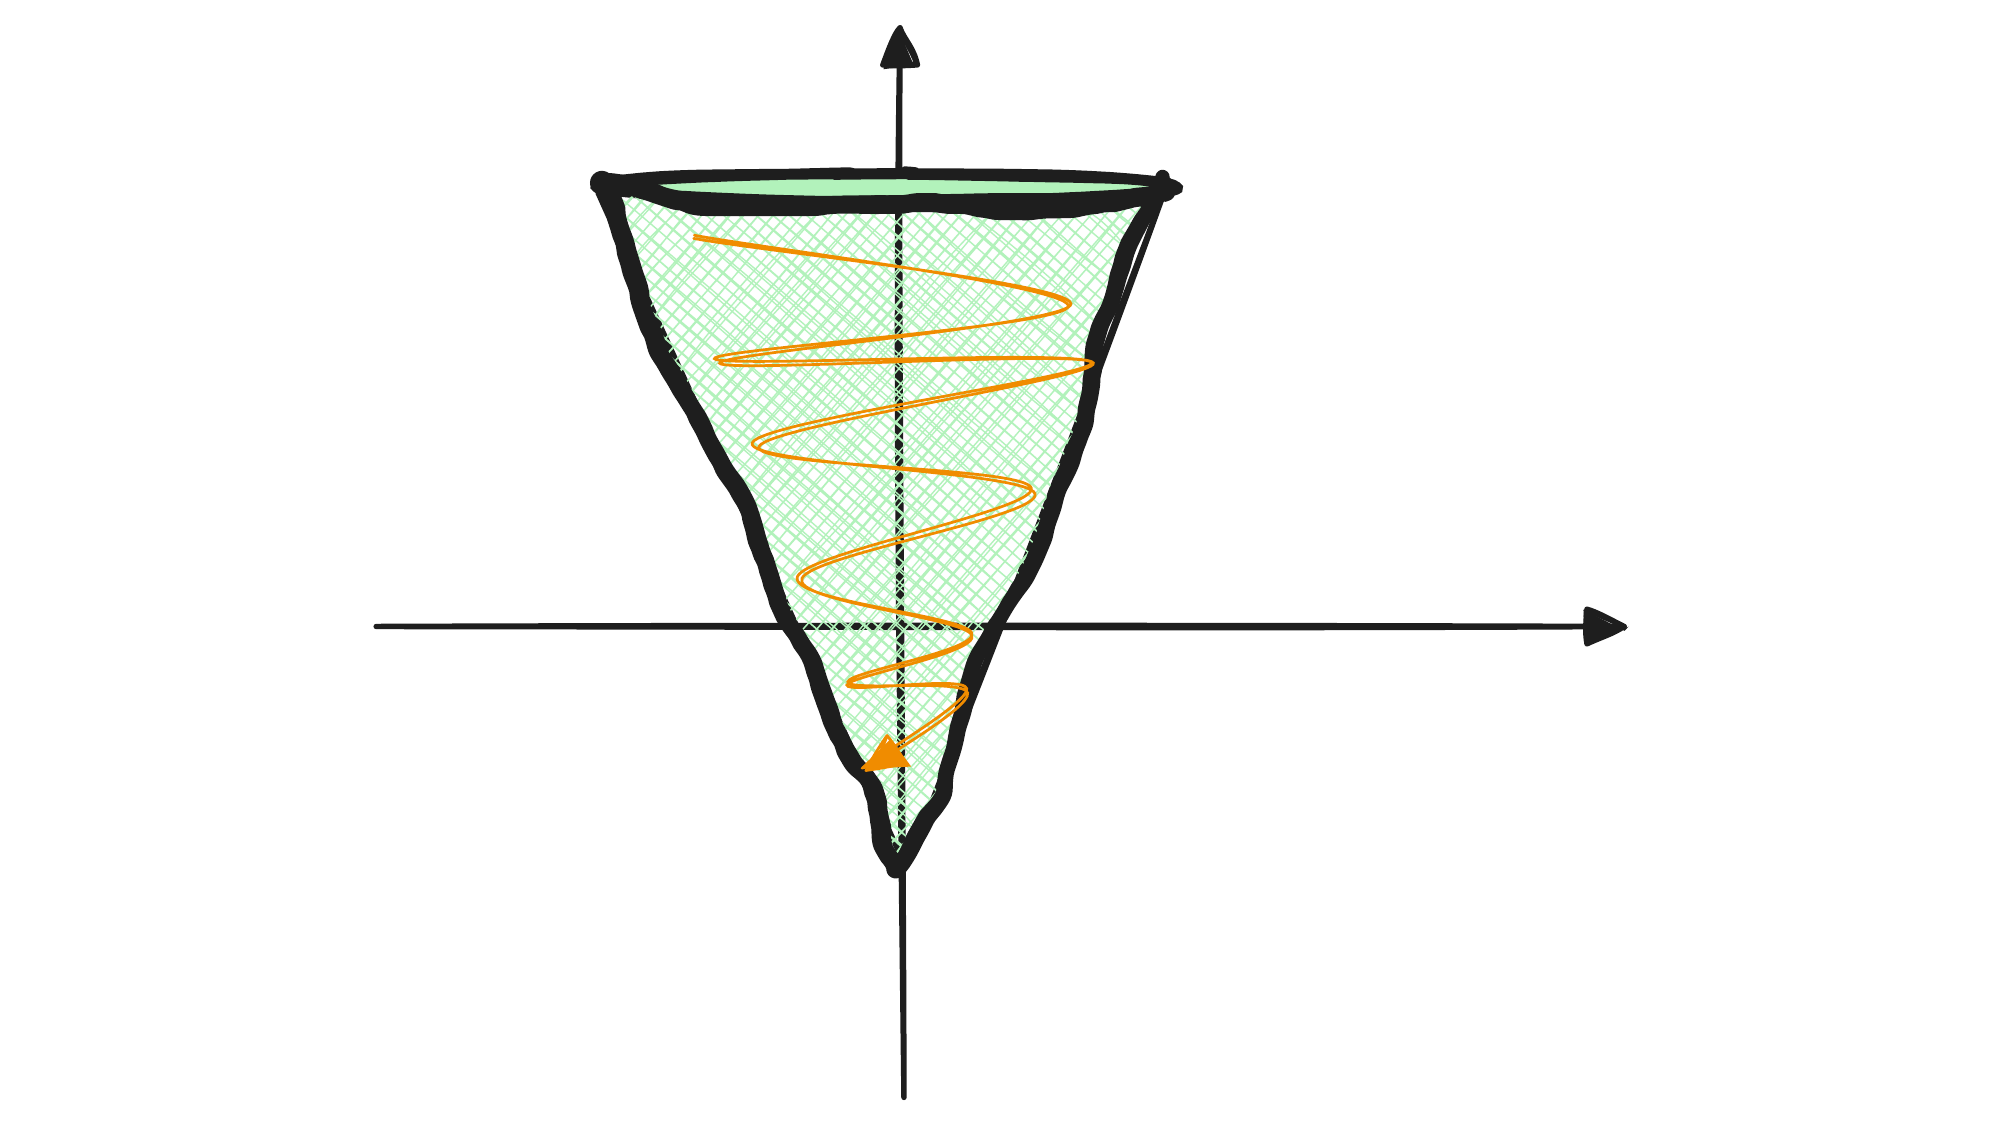}
    \caption{TODO add stuff}
    \label{fig:coneFailedAttempt}
\end{figure}

and...

\begin{figure}
    \centering
    \includegraphics[width=0.6\textwidth]{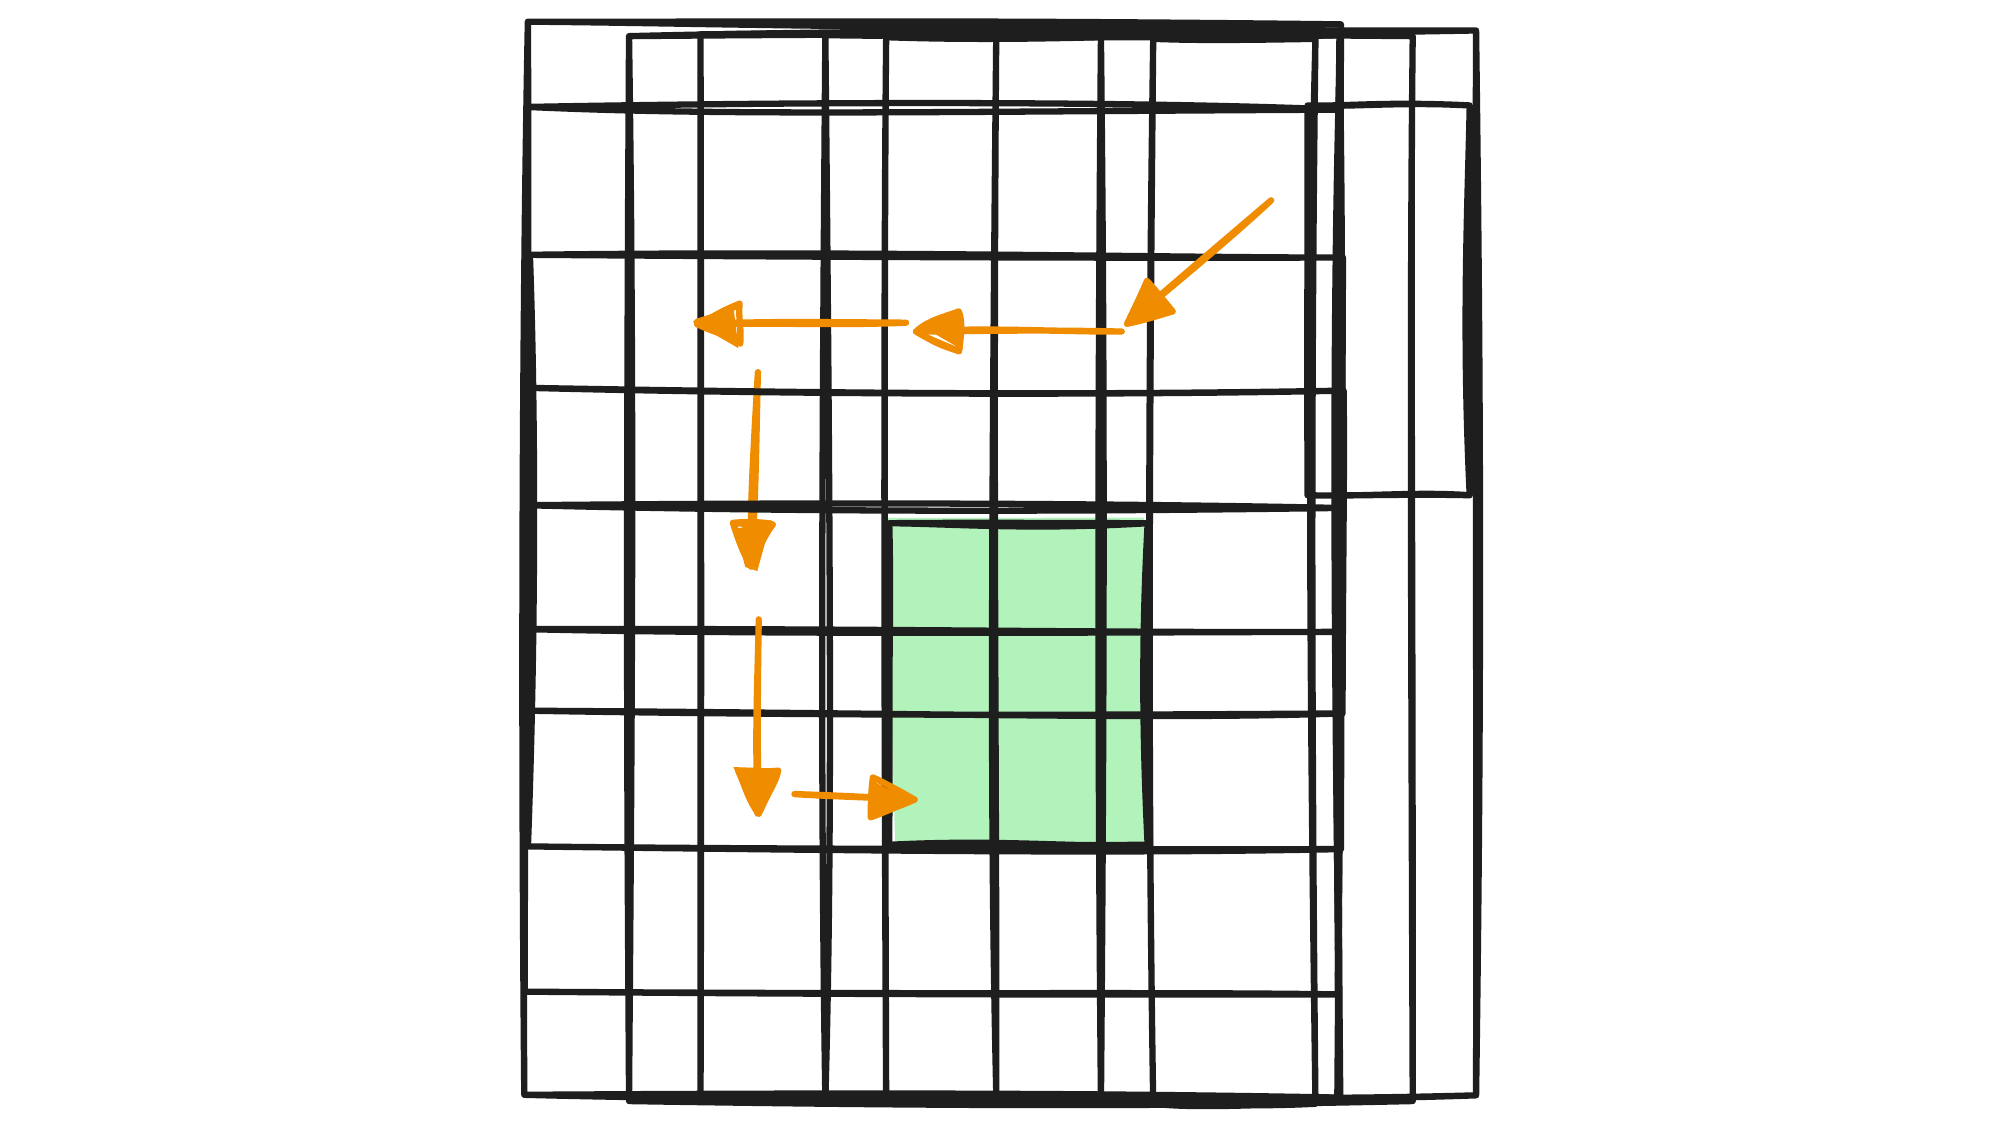}
    \caption{TODO add stuff}
    \label{fig:gridFailedAttempt}
\end{figure}

%Ieva
\newpage
\section{$K$-induction based verification. The structure of re-designed neural network.}
\label{sec:appendix:k_ind_nn}

\begin{figure}[h]
    \centering
    \includegraphics[width=0.2\textwidth]{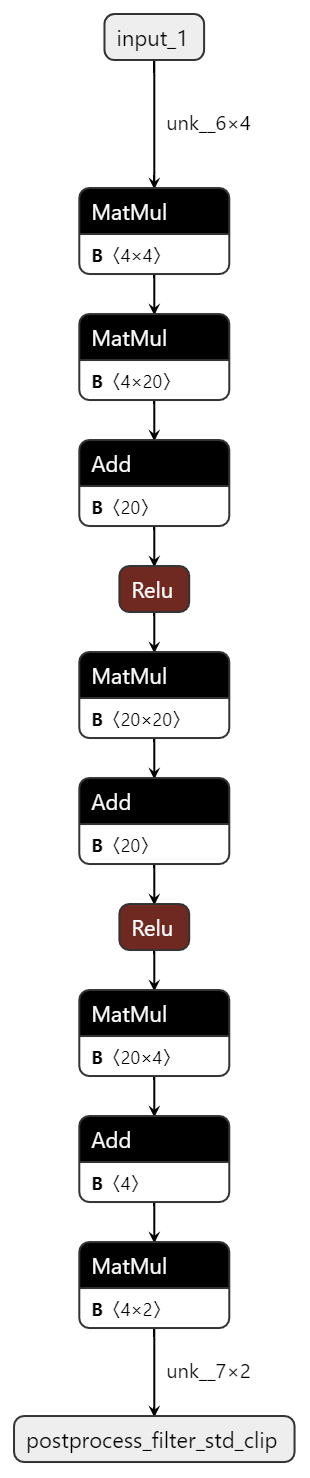}
    \caption{Visualized architecture of the redesigned neural network controller.\newline}
    \label{sec:appendix:onnx}
\end{figure}

The visualization of the retrained deep learning model reflects the structure and the data flow of the model, its layers and how they are connected. Each box represents a layer in the neural network. The upper and lower parts of the box indicate the layer type and the number of units (or filters) accordingly. \textbf{Input and output nodes}. Input box represents the shape of the input data (for example, $4\times4$ input is the 4 dimensional state. Output box represents the shape of the output data. For example, dimensions $unk\_7\times2$ are batch size of 7 and the output size of 2 (which is thrust on $x$ and $y$, components of the force). \textbf{Arrows} represent the connections between the layers and the direction of data flow.
% generated with netron.app

%Ieva
\newpage
\section{Deriving the space motion dynamics equations for the Polar coordinate system}
\label{sec:appendix:polar}

Given the polar coordinates $r$ (the radial coordinate, the radial distance from the origin) and $\theta$ (the angular coordinate, also called the polar angle, the counterclockwise angle from the x-axis), Cartesian coordinates can be defined as:

\begin{align}
    x = r \cos \theta\\
    y = r \sin \theta
\end{align}

and polar coordinates can be defined\footnote{\url{https://en.wikipedia.org/wiki/Polar_coordinate_system}} in terms of x and y as:

\begin{align}
    r = \sqrt{x^2 + y^2}\\
    \theta = \tan ^{-1} \frac{y}{x}
\end{align}. 

% equations for polar
\includepdf[pages=-, scale=0.8]{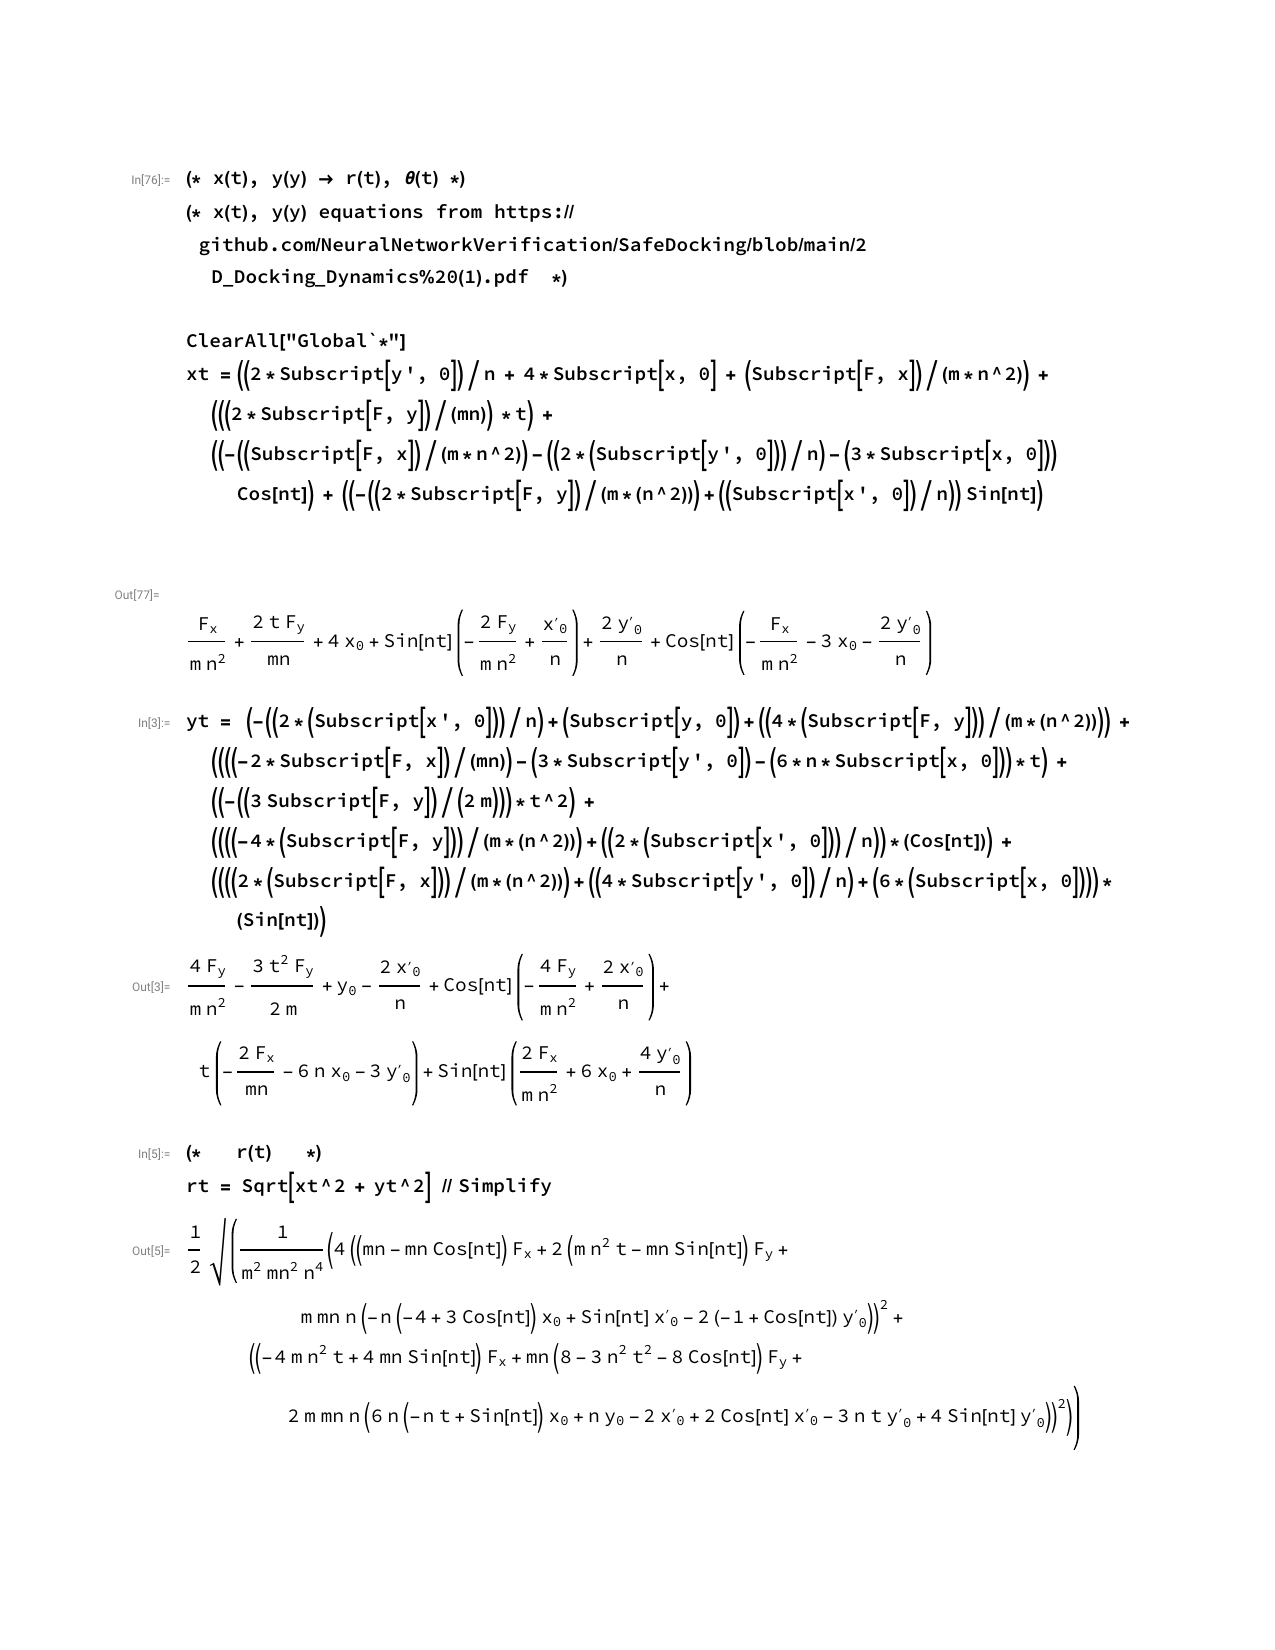}

% empirical comparison Cartesian NN vs Polar NN docking
\begin{figure}[h]
    \centering
\begin{subfigure}[b]{0.30\textwidth}
\includegraphics[width=\textwidth]
{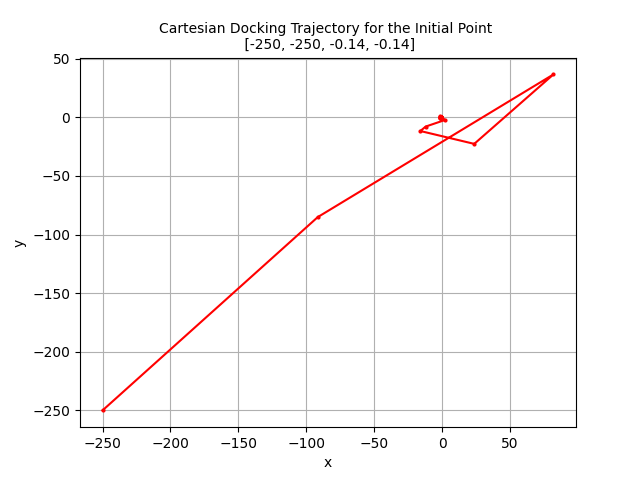}
\caption{Original (Cartesian) neural network.}
\label{fig:cartesian_nn}
\end{subfigure}
\begin{subfigure}[b]{0.30\textwidth} \includegraphics[width=\textwidth]{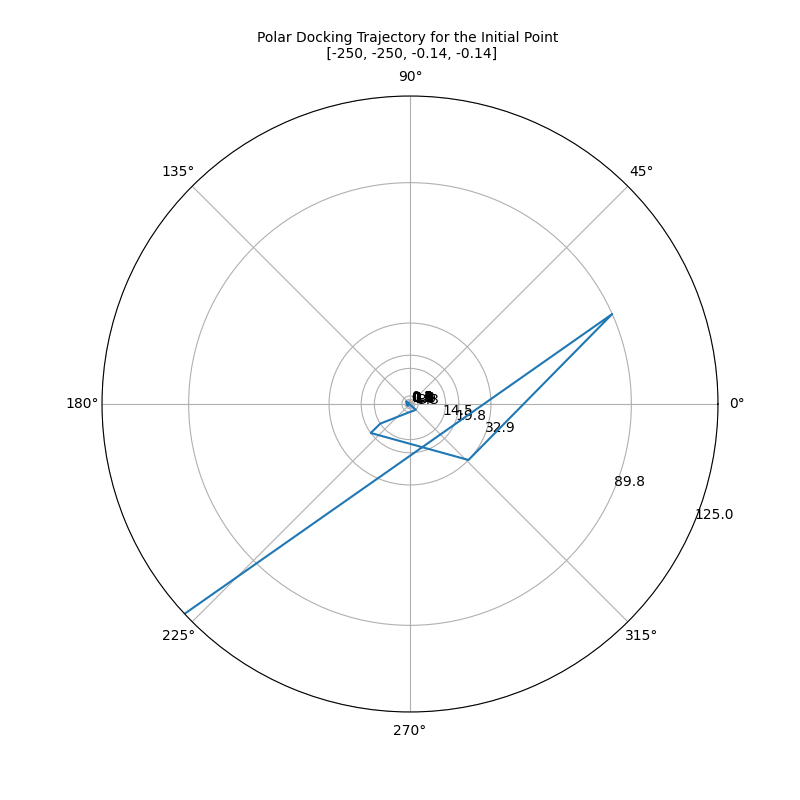}    
\caption{Re-designed (Polar) neural network.}  
\label{fig:polar_nn}
\end{subfigure} \caption{Design for Verification. Empirical comparison of neural network controllers' trajectories for a given initial state: original Cartesian vs Polar systems.}
\label{fig:cartesian_vs_polar}
\end{figure}

% k values for polar
\begin{figure}[h]
    \centering
\begin{subfigure}[b]{0.30\textwidth}
\includegraphics[width=\textwidth]
{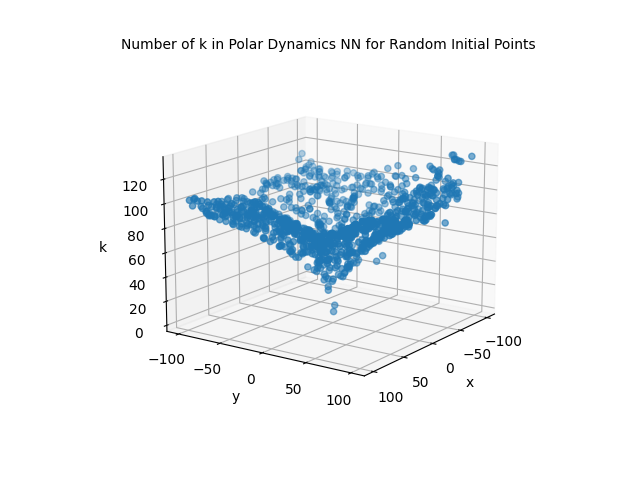}
\caption{Polar dynamics. Number of \textit{k} for random initial points.}
\label{fig:polar_k_init}
\end{subfigure}
\begin{subfigure}[b]{0.30\textwidth} \includegraphics[width=\textwidth]{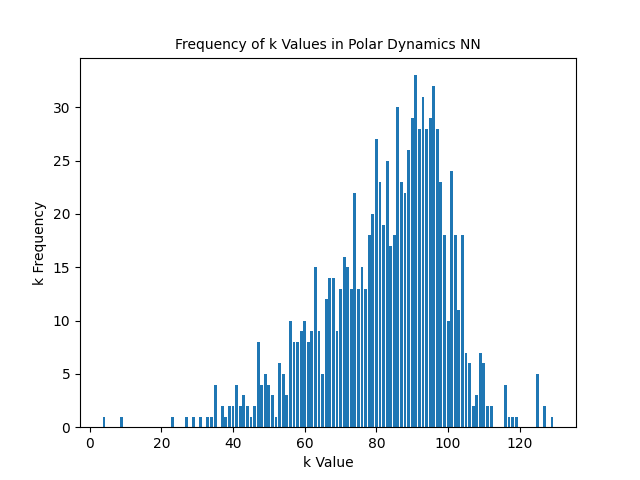}    
\caption{Frequency of \textit{k} values.}  
\label{fig:polar_k_freq}
\end{subfigure} \caption{Polar system's verification. Scalability perspective evaluation by \textit{k}, the number of instances where the current coordinate is closer to the chief than the preceding coordinate. 1010 experiments ($x, y \in [-100,100], k_{max} = 129, k_{min} = 4, k_{avg} = 82$).}
\label{fig:polar_k}
\end{figure}

% sim_env for polar 
\begin{figure}[h]
    \centering
\begin{subfigure}[b]{0.50\textwidth}
\includegraphics[width=\textwidth]
{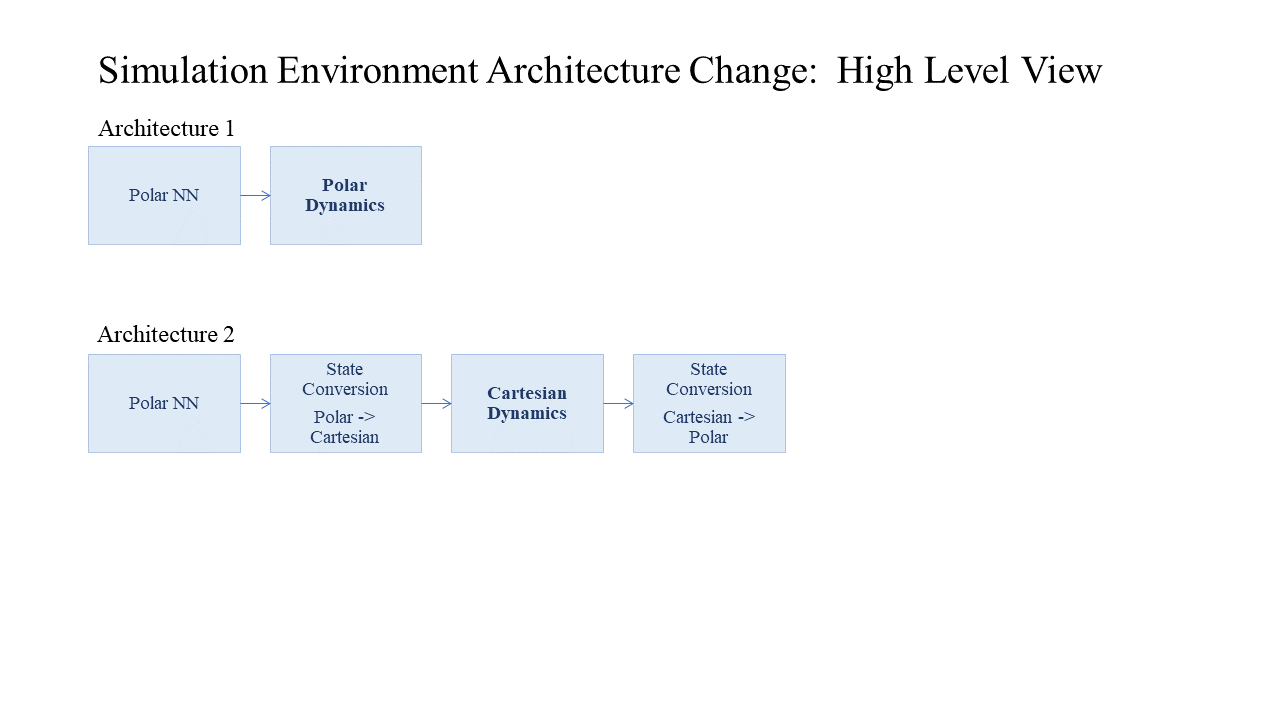}
\caption{Polar system's software architecture comparison to Cartesian system. A high level overview.\\}
\label{fig:sim_env_polar_1}
\end{subfigure}
\begin{subfigure}[b]{0.50\textwidth} \includegraphics[width=\textwidth]{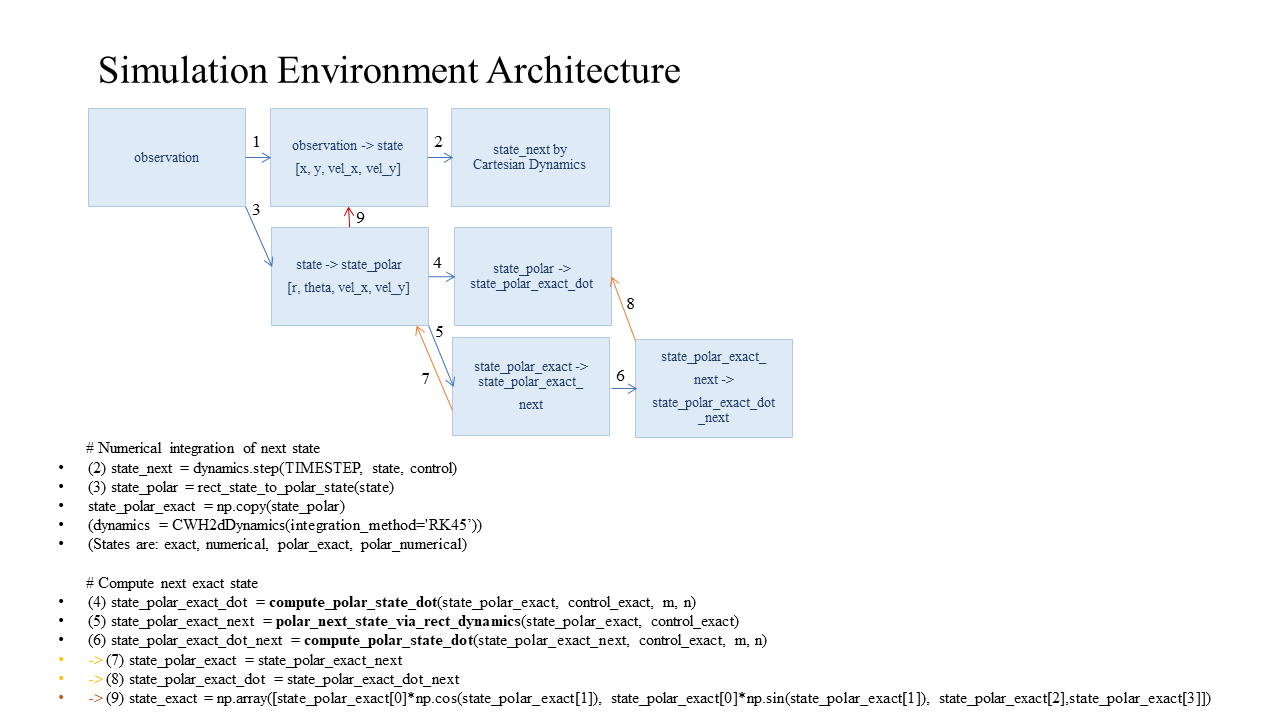}    
\caption{Polar system's architecture. Numerical integration of the next state (steps 2, 3) and computation of the next exact state (steps 4-9).}  
\label{fig:sim_env_polar_2}
\end{subfigure} \caption{Polar system's Simulation Environment Architecture. High level and in detail diagrams.}
\label{fig:sim_env_polar}
\end{figure}

% Overt: linearizing r 
\begin{figure}[h]
    \centering
\begin{subfigure}[b]{0.40\textwidth}
\includegraphics[width=\textwidth]
{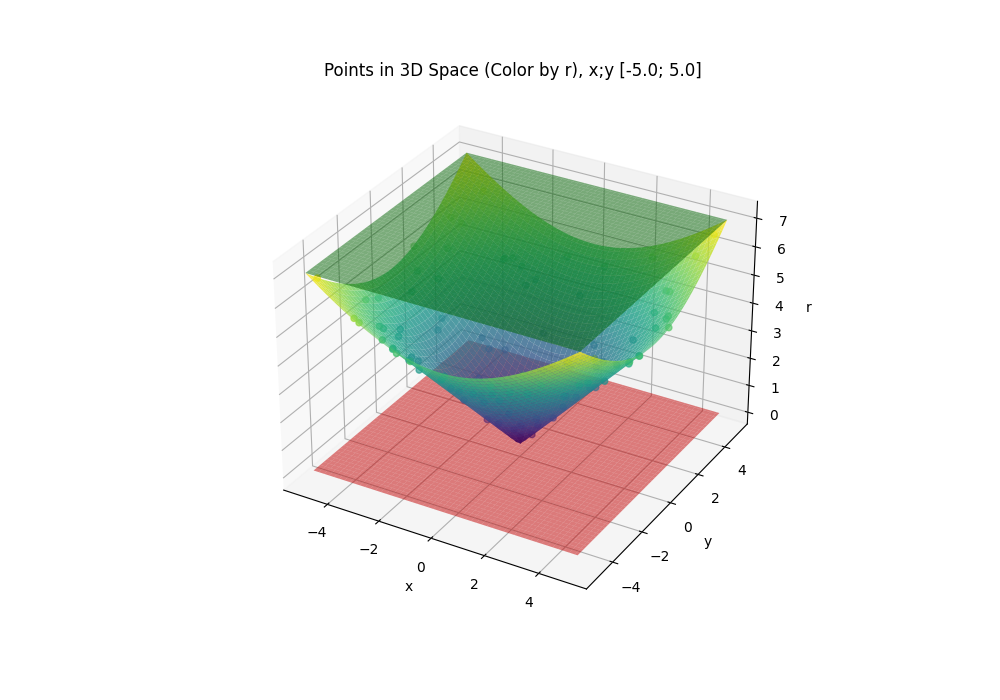}
\caption{Approximating $r = sqrt(x^2 + y^2)$; OVERT approximated $r_{min} = 0.122, r_{max} = 7.072$.\\}
%$r_{min} = 0.12178775797650376, r_{max} = 7.0721161088597055$.
\label{fig:overt_1}
\end{subfigure}
\begin{subfigure}[b]{0.40\textwidth} \includegraphics[width=\textwidth]{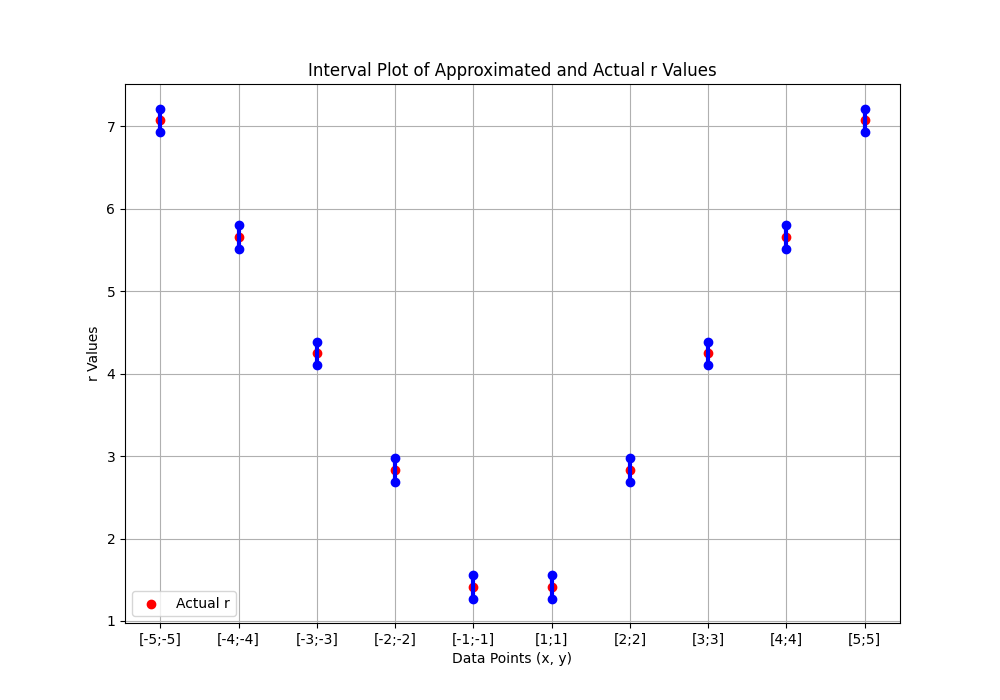}    
\caption{Comparison Graph: Approximated vs Actual $r$.}  
\label{fig:overt_2}
\end{subfigure} \caption{Julia OVERT performance on the linear approximation task. Polar coordinate $r$ values for $x,y \in [-5.0,-0.1]\cup(0.1,5.0]$}
\label{fig:overt}
\end{figure}
